# Supplementary material for: Probing exotic cross-shell interactions at N=28 with single-neutron transfer on 47K
Source: arXiv:2409.12594 source file (2025-01-08)
Supplement: Supplementary file 1 [file 47Kdp_Dec2024_Supplemental.pdf]

# Supplement to "Probing exotic cross-shell interactions at $N = 28$ with single-neutron transfer on $^{47}$K"


C. J. Paxman,[1] A. Matta,[2] W. N. Catford,[1] G. Lotay,[1] M. Assié,[3] E. Clément,[4] A. Lemasson,[4] D. Ramos,[4] N. A. Orr,[2] F. Galtarossa,[3] V. Girard-Alcindor,[4] J. Dudouet,[5] N. L. Achouri,[2] D. Ackermann,[4] D. Barrientos,[6] D. Beaumel,[3] P. Bednarczyk,[7] G. Benzoni,[8] A. Bracco,[8,9] L. Canete,[1] B. Cederwall,[10] M. Ciemala,[7] P. Delahaye,[4] D. T. Doherty,[1] C. Domingo-Pardo,[11] B. Fernández-Domínguez,[12] D. Fernández,[12] F. Flavigny,[2] C. Fougères,[4] G. de France,[4] S. Franchoo,[3] A. Gadea,[11] J. Gibelin,[2] V. González,[13] A. Gottardo,[14] N. Goyal,[4] F. Hammache,[3] L. J. Harkness-Brennan,[15] D. S. Harrouz,[3] B. Jacquot,[4] D. S. Judson,[15] A. Jungclaus,[16] A. Kaşkaş,[17] W. Korten,[18] M. Labiche,[19] L. Lalanne,[3,4] C. Lenain,[2] S. Leoni,[8,9] J. Ljungvall,[3] J. Lois-Fuentes,[12] T. Lokotko,[2] A. Lopez-Martens,[3] A. Maj,[7] F. M. Marqués,[2] I. Martel,[20] R. Menegazzo,[21] D. Mengoni,[21,22] B. Million,[8] J. Nyberg,[23] R. M. Pérez-Vidal,[11,14] L. Plagnol,[2] Zs. Podolyák,[1] A. Pullia,[8,9] B. Quintana,[24] D. Regueira-Castro,[12] P. Reiter,[25] M. Rejmund,[4] K. Rezynkina,[26,21] E. Sanchis,[13] M. Şenyiğit,[17] N. de Séréville,[3] M. Siciliano,[14,18,27] D. Sohler,[28] O. Stezowski,[5] J.-C. Thomas,[4] A. Utepov,[4] J. J. Valiente-Dobón,[14] D. Verney,[3] and M. Zielińska[18]

[1]*School of Maths and Physics, University of Surrey, Guildford, GU2 7XH, United Kingdom*
[2]*Université de Caen Normandie, ENSICAEN, CNRS/IN2P3, LPC Caen UMR6534, F-14000 Caen, France*
[3]*Université Paris-Saclay, CNRS/IN2P3, IJCLab, 91405 Orsay, France*
[4]*Grand Accélérateur National d'Ions Lourds (GANIL), CEA/DRF-CNRS/IN2P3, Bvd Henri Becquerel, 14076 Caen, France*
[5]*Université Claude Bernard Lyon 1, CNRS/IN2P3, IP2I Lyon, UMR 5822, F-69100 Villeurbanne, France*
[6]*CERN, CH-1211 Geneva 23 (Switzerland)*
[7]*The Henryk Niewodniczański Institute of Nuclear Physics, Polish Academy of Sciences, ul. Radzikowskiego 152, 31-342 Kraków, Poland*
[8]*INFN Sezione di Milano, I-20133 Milano, Italy*
[9]*Dipartimento di Fisica, Università di Milano, I-20133 Milano, Italy*
[10]*Department of Physics, KTH Royal Institute of Technology, SE-10691 Stockholm, Sweden*
[11]*Instituto de Física Corpuscular, CSIC-Universidad de Valencia, E-46071 Valencia, Spain*
[12]*IGFAE and Dpt. de Física de Partículas, Univ. of Santiago de Compostela, E-15758, Santiago de Compostela, Spain*
[13]*Departamento de Ingeniería Electrónica, Universitat de Valencia, Burjassot, Valencia, Spain*
[14]*Laboratori Nazionali di Legnaro, INFN, I-35020 Legnaro (PD), Italy*
[15]*Oliver Lodge Laboratory, The University of Liverpool, Liverpool, L69 7ZE, UK*
[16]*Instituto de Estructura de la Materia, CSIC, Madrid, E-28006 Madrid, Spain*
[17]*Department of Physics, Faculty of Science, Ankara University, 06100 Besevler - Ankara, Turkey*
[18]*Irfu, CEA, Université Paris-Saclay, F-91191 Gif-sur-Yvette, France*
[19]*STFC Daresbury Laboratory, Daresbury, Warrington, WA4 4AD, UK*
[20]*Departamento de Ciencias Integradas, Universidad de Huelva, Calle Dr. Cantero Cuadrado, 6, 21004 Huelva, Spain*
[21]*INFN Sezione di Padova, I-35131 Padova, Italy*
[22]*Dipartimento di Fisica e Astronomia dell'Università di Padova, I-35131 Padova, Italy*
[23]*Department of Physics and Astronomy, Uppsala University, SE-75120 Uppsala, Sweden*
[24]*Laboratorio de Radiaciones Ionizantes, Departamento de Física Fundamental, Universidad de Salamanca, E-37008 Salamanca, Spain*
[25]*Institut für Kernphysik, Universität zu Köln, Zülpicher Str. 77, D-50937 Köln, Germany*
[26]*Université de Strasbourg, CNRS, IPHC UMR 7178, F-67000 Strasbourg, France*
[27]*Physics Division, Argonne National Laboratory, Lemont (IL), United States*
[28]*Institute for Nuclear Research, Atomki, 4001 Debrecen, P.O. Box 51, Hungary*



(Dated: December 19, 2024)


In Fig. 1, we present a full level scheme diagram of $^{48}$K, as populated by the $^{47}$K(d,p) single-neutron transfer reaction. This figure repeats the experimental information presented in Table I and is provided here as a visual aid to the reader.

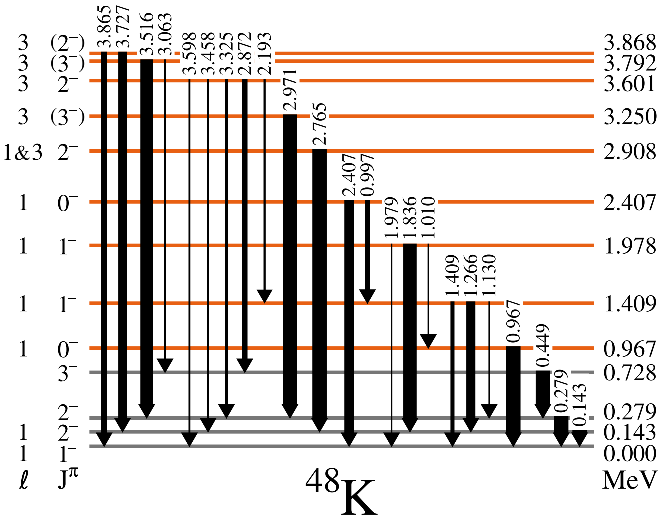


FIG. 1. Level scheme of $^{48}$K determined in this work. Previously known states are in grey, with new states in orange. For each state, the $\ell$-transfer and spin-parity ($J^{\pi}$) are indicated to the left, and the energy (in MeV) is given on the right. The $\gamma$-ray transitions are indicated with black arrows (where the thickness of the arrow indicates the branching ratio) and are labeled with their energy.
